# Supplementary material for: Safe Non-Stochastic Control of Linear Dynamical Systems
Source: arXiv:2308.12395 source file (2023-08-23)
Supplement: Supplementary file 1 [file Appendix-SAder.tex]

\subsection{Proof of \Cref{theorem:SafeAder}}\label{app:theorem_SafeAder}
\begin{proof}
First, since each base-learner $\calB_i$ performs \SafeOGD with step size $\eta_i$ over surrogate loss $\ell_t$ , we have
\begin{equation}
    \sum_{t=1}^T \ell_t\left(\mathbf{x}_{t,i}\right)-\sum_{t=1}^T \ell_t\left(\mathbf{v}_t\right) \leq \frac{7 D^2}{4 \eta_i} + \frac{D}{\eta_i} C_T + \frac{D}{\eta_i} S_T + \frac{\eta_i T}{2} G^2.
    \label{eq:theorem_SafeAder_1}
\end{equation}

The optimal step size $\eta^\star$ that minimizes the dynamic regret bound in \cref{eq:theorem_SafeAder_1} is 
\begin{equation}
    \eta^\star = \sqrt{\frac{7 D^2 + 4 D C_T + 4 D S_T}{2 T G^2}} .
    \label{eq:theorem_SafeAder_2}
\end{equation}

By \Cref{assumption:bounded_set}, we have the following bound of the $C_T$ and $S_T$,
\begin{equation}
    \begin{aligned}
        0 & \leq C_T = \sum_{t=2}^T\left\|\mathbf{v}_t-\mathbf{v}_{t-1}\right\| \leq T D \\
        0 & \leq S_T = \sum_{t=1}^T\left\|\bar{\myx}_{t+1} - {\myx}_{t+1} \right\| \leq T D .
    \label{eq:theorem_SafeAder_3}
    \end{aligned}
\end{equation}

Thus, the optimal step size satisfies
\begin{equation}
    \frac{D}{G} \sqrt{\frac{7}{2 T}} \leq \eta^\star \leq \frac{D}{G} \sqrt{\frac{7}{2 T} + 4} .
    \label{eq:theorem_SafeAder_4}
\end{equation}

From the definition of $\mathcal{H}$ in \cref{eq:SafeAder_step_size_pool}, we have $\min \mathcal{H}=\frac{D}{G} \sqrt{\frac{7}{2 T}}$ and $\max \mathcal{H} \geq \frac{D}{G} \sqrt{\frac{7}{2 T}+4}$. Hence, there exists a step size $\eta_k \in \calH$ such that 
\begin{equation}
    \eta_k = \frac{2^{k-1} D}{G} \sqrt{\frac{7}{2 T}} \leq \eta^\star \leq  2 \eta_k,
    \label{eq:theorem_SafeAder_5}
\end{equation}
where $k=\left\lfloor\frac{1}{2} \log _2\left(1+\frac{4 C_T + 4 S_T}{7 D}\right)\right\rfloor+1$.

Substituting $\eta_k$ into \cref{eq:theorem_SafeAder_1} and using \cref{eq:theorem_SafeAder_2,eq:theorem_SafeAder_5} gives
\begin{equation}
    \begin{aligned}
        \sum_{t=1}^T \ell_t\left(\mathbf{x}_{t,k}\right)-\sum_{t=1}^T \ell_t\left(\mathbf{v}_t\right) &\leq \frac{7 D^2}{4 \eta_k} + \frac{D}{\eta_k} C_T + \frac{D}{\eta_k} S_T + \frac{\eta_k T}{2} G^2 \\
        & \leq  \frac{7 D^2}{2 \eta^\star} + \frac{2D}{\eta^\star} C_T + \frac{2D}{\eta^\star} S_T + \frac{\eta^\star T}{2} G^2 \\
        & =  \frac{3}{4}\sqrt{2 T G^2 (7 D^2 + 4 D C_T + 4 D S_T)}.
    \label{eq:theorem_SafeAder_6}
    \end{aligned}
\end{equation}

Next, we analyze the regret of \Hedge via the following lemma.
\begin{lemma}\citep[Lemma~3]{zhang2018adaptive}\label{lemma:hedge}
    The regret of \Hedge satisfies
    \begin{equation}
        \sum_{t=1}^T \ell_t\left(\myx_t\right)-\min _{i}\left(\sum_{t=1}^T \ell_t\left(\myx_{t,i}\right)+\frac{1}{\epsilon} \ln \frac{1}{p_{1,i}}\right) \leq \frac{\epsilon T G^2 D^2}{2} ,
    \label{eq:lemma_hedge_1}
    \end{equation}
    where $i \in \{1,\dots,N\}$.
\end{lemma}

By choosing $\epsilon=\sqrt{2 /\left(T G^2 D^2\right)}$ to minimize the upper bound in \cref{eq:lemma_hedge_1}, we have for the base-learner $\calB_k$
\begin{equation}
    \sum_{t=1}^T \ell_t\left(\mathbf{x}_t\right)-\sum_{t=1}^T \ell_t\left(\mathbf{x}_{t,k}\right) \leq \frac{\sqrt{2 T} G D }{2}\left(1+\ln \frac{1}{p_{1,k}}\right).
    \label{eq:theorem_SafeAder_7}
\end{equation}

From \cref{eq:SafeAder_initial_weight}, the initial weight of the base-learner $\calB_k$ satisfies
\begin{equation}
    p_{1,k} = \frac{1}{k(k+1)}\cdot\frac{N+1}{N} \geq \frac{1}{k(k+1)} \geq \frac{1}{(k+1)^2} .
    \label{eq:theorem_SafeAder_8}
\end{equation}

Substituting \cref{eq:theorem_SafeAder_8} into \cref{eq:theorem_SafeAder_7}
\begin{equation}
    \sum_{t=1}^T \ell_t\left(\mathbf{x}_t\right)-\sum_{t=1}^T \ell_t\left(\mathbf{x}_{t,k}\right) \leq \frac{\sqrt{2 T} G D }{2}\left(1 + 2\ln (k+1)\right).
    \label{eq:theorem_SafeAder_9}
\end{equation}

Combining \cref{eq:theorem_SafeAder_6,eq:theorem_SafeAder_9}, we have
\begin{equation}
    \sum_{t=1}^T \ell_t\left(\mathbf{x}_t\right)-\sum_{t=1}^T \ell_t\left(\mathbf{v}_t\right) \leq \frac{3}{4}\sqrt{2 T G^2 (7 D^2 + 4 D C_T + 4 D S_T)} + \frac{\sqrt{2 T} G D }{2}\left(1 + 2\ln (k+1)\right).
    \label{eq:theorem_SafeAder_10}
\end{equation}

Since
\begin{equation}
    \begin{aligned}
     f_t\left(\mathbf{x}_t\right) - f_t\left(\mathbf{v}_t\right)  &\leq  \left\langle\nabla f_{t}\left(\mathbf{x}_{t}\right), \mathbf{x}_{t}-\mathbf{v}_{t}\right\rangle \\
     &= \left\langle\nabla f_{t}\left(\mathbf{x}_{t}\right), \mathbf{x}_{t}-\mathbf{x}_{t}\right\rangle - \left\langle\nabla f_{t}\left(\mathbf{x}_{t}\right), \mathbf{v}_{t}-\mathbf{x}_{t}\right\rangle \\
     &= \ell_t\left(\mathbf{x}_t\right) - \ell_t\left(\mathbf{v}_t\right),
    \end{aligned}
\end{equation}
we thus have
\begin{equation}
    \sum_{t=1}^T f_t\left(\mathbf{x}_t\right)-\sum_{t=1}^T f_t\left(\mathbf{v}_t\right) \leq \frac{3}{4}\sqrt{2 T G^2 (7 D^2 + 4 D C_T + 4 D S_T)} + \frac{\sqrt{2 T} G D }{2}\left(1 + 2\ln (k+1)\right), 
\end{equation}
which holds for any sequence of comparators $(\mathbf{v}_1, \dots, \mathbf{v}_T) \in \calX_1 \times \cdots \times \calX_T$. 
\end{proof}

\subsection{Proof of \Cref{lemma:hedge}}
\begin{proof}
Following \citep[Theorem~2.2, Exercise~2.5]{cesa2006prediction}, we define
\begin{equation}
    \begin{aligned}
        L_{t,i} &= \sum_{\tau=1}^t \ell_{\tau}\left(\mathbf{x}_{\tau,i}\right), \\
        W_t &= \sum_{i=1}^N p_{1,i} e^{-\epsilon L_{t,i}} .    
    \label{eq:lemma_hedge_2}
    \end{aligned}
\end{equation}

From line 8 in \Cref{alg:SafeAder}, we have for $t \geq 2$,
\begin{equation}
    \begin{aligned}
        p_{t,i}=\frac{p_{1,i} e^{-\epsilon L_{t-1,i}}}{\sum_{j=1}^N p_{1,j} e^{-\epsilon L_{t-1,j}}}.
    \end{aligned}
    \label{eq:lemma_hedge_3}
\end{equation}

First, we have
\begin{equation}
    \begin{aligned}
        \ln W_T &= \ln \left(\sum_{i=1}^N p_{1,i} e^{-\epsilon L_{t,i}}  \right) \geq \ln \left(\max_{i} \  p_{1,i} e^{-\epsilon L_{t,i}}\right)=-\epsilon \min_{i} \left(L_{t,i}+\frac{1}{\epsilon} \ln \frac{1}{p_{1,i}}\right), \\
        \ln W_1 &= \ln \left(\sum_{i=1}^N p_{1,i} e^{-\epsilon \ell_1\left(\mathbf{x}_{1,i}\right)}\right)
    \end{aligned}
    \label{eq:lemma_hedge_4}
\end{equation}

For $t \geq 2$, we have
\begin{equation}
    \begin{aligned}
    \ln \left(\frac{W_t}{W_{t-1}}\right) &= \ln \left(\frac{\sum_{i=1}^N p_{1,i} e^{-\epsilon L_{t,i}}}{\sum_{i=1}^N p_{1,i} e^{-\epsilon L_{t-1,i}}}\right) \\
    &= \ln \left(\frac{\sum_{i=1}^N p_{1,i} e^{-\epsilon L_{t-1,i}} e^{-\epsilon \ell_t\left(\mathbf{x}_{t,i}\right)}}{\sum_{i=1}^N p_{1,i} e^{-\epsilon L_{t-1,i}}}\right) \\
    &= \ln \left(\sum_{i=1}^N p_{t,i} e^{-\epsilon \ell_t\left(\mathbf{x}_{t,i}\right)}\right),
    \end{aligned}
    \label{eq:lemma_hedge_5}
\end{equation}
where the last equality holds by substituting \cref{eq:lemma_hedge_3}.

Combining \cref{eq:lemma_hedge_4,eq:lemma_hedge_5} gives
\begin{equation}
    \ln W_T=\ln W_1+\sum_{t=2}^T \ln \left(\frac{W_t}{W_{t-1}}\right) = \sum_{t=1}^T \ln \left(\sum_{i=1}^N p_{t,i} e^{-\epsilon \ell_t\left(\mathbf{x}_{t,i}\right)}\right) .
    \label{eq:lemma_hedge_6}
\end{equation}

By the Cauchy-Schwarz inequality, \Cref{assumption:bounded_set}, and \Cref{assumption:gradient}, the surrogate loss can be bounded as
\begin{equation}
    \begin{aligned}
        {\ell}_t(\mathbf{x})&=\left\langle \nabla {f}_{t}\left(\mathbf{x}_{t}\right), \mathbf{x}-\mathbf{x}_{t}\right\rangle \leq \left\| \nabla {f}_{t}\left(\mathbf{x}_{t}\right) \right\| \left\| \mathbf{x}-\mathbf{x}_{t} \right\| \leq GD, \\
        -{\ell}_t(\mathbf{x})&=\left\langle \nabla {f}_{t}\left(\mathbf{x}_{t}\right), \mathbf{x}_{t} -\mathbf{x}\right\rangle \leq \left\| \nabla {f}_{t}\left(\mathbf{x}_{t}\right) \right\| \left\| \mathbf{x}_{t}-\mathbf{x} \right\| \leq GD.
    \end{aligned}
    \label{eq:lemma_hedge_7}
\end{equation}

Using Hoeffding’s inequality \cite{hoeffding1994probability} and \cref{eq:lemma_hedge_7}, we obtain
\begin{equation}
    \begin{aligned}
        \ln \left(\sum_{i=1}^N p_{t,i} e^{-\epsilon \ell_t\left(\mathbf{x}_{t,i}\right)}\right) & \leq-\epsilon \sum_{i=1}^N p_{t,i} \ell_t\left(\mathbf{x}_{t,i}\right)+\frac{\epsilon^2 G^2 D^2}{2} \\
    & \leq-\epsilon \ell_t\left(\sum_{i=1}^N p_{t,i} \mathbf{x}_{t,i}\right)+\frac{\epsilon^2 G^2 D^2}{2} \\
    & = -\epsilon \ell_t\left(\mathbf{x}_t\right)+\frac{\epsilon^2 G^2 D^2}{2} .
    \end{aligned}
    \label{eq:lemma_hedge_8}
\end{equation}
where the second inequality holds due to Jensen's inequality \cite{boyd2004convex}. 

Substituting \cref{eq:lemma_hedge_8} into \cref{eq:lemma_hedge_7}, we obtain
\begin{equation}
    \ln W_T \leq-\epsilon \sum_{t=1}^T \ell_t\left(\mathbf{x}_t\right)+\frac{ \epsilon^2 T G^2 D^2}{2} .
    \label{eq:lemma_hedge_9}
\end{equation}

Combining \cref{eq:lemma_hedge_9} with the lower bound of $\ln W_T$ in \cref{eq:lemma_hedge_4}, we have
\begin{equation}
    -\epsilon \min _{i}\left(L_{t,i}+\frac{1}{\epsilon} \ln \frac{1}{p_{1,i}}\right) \leq-\epsilon \sum_{t=1}^T \ell_t\left(\mathbf{x}_t\right)+\frac{\epsilon^2 T G^2 D^2}{2} .
    \label{eq:lemma_hedge_10}
\end{equation}

Simplifying \cref{eq:lemma_hedge_10} gives \cref{eq:lemma_hedge_1}.
\end{proof}
