# Supplementary material for: Safe Non-Stochastic Control of Linear Dynamical Systems
Source: arXiv:2308.12395 source file (2023-08-23)
Supplement: Supplementary file 2 [file Appendix-Exp.tex]

\section{Supplementary Numerical Experiments}\label{app:supp_exp}
\input{Table/Table-OCOvsOCOM.tex}

We compare \Cref{alg:SafeOGD_Control} and \Cref{alg:SafeAder_Control} with state-of-the-art \OCOM controllers in simulated scenarios of online control of linear time-invariant systems with constraints on control inputs. 

\myParagraph{Compared Algorithms} 
We compare \SafeOGD and \SafeAder controllers with the \DAC \citep{agarwal2019online} and \Scream \citep{zhao2022non} controllers.

\myParagraph{Simulation Setup} 
We follow the setup similar to \cite{zhao2022non}. We consider linear systems of the form
\begin{equation}\label{eq:aux_exp}
    \begin{aligned}
        x_{t+1} &= A x_{t} + B u_{t} + w_{t},
    \end{aligned}
\end{equation}
    where $x_t \in \mathbb{R}^2$, $u_t\in \mathbb{R}$, ${w}_{t}$ and the elements of $A$ and $B$ matrices are sampled from various distributions, \ie Gaussian, Uniform, Gamma, Beta, Exponential, and Weibull distributions. For \SafeOGD and \DAC controllers, we use two different step sizes for each controller: the first and the fourth step size in the step size pool of \SafeAder and \Scream controllers respectively, \ie $\eta_1$ and $\eta_4$. The loss function for \DAC and \Scream controllers has the form $c_t(x_{t},u_t) = 
 q_t x_t^\top x_t + r_t u_t^\top u_t$, where $q_t$, $r_t \in \mathbb{R}$ are time-varying weights. Particularly, we consider two cases:
 
%  \red{after finalizing, fix extra white space, if still any}
 
\begin{enumerate}%[leftmargin=9pt]\setlength\itemsep{-1.mm}
    \item Sinusoidal weights defined as 
    \begin{equation}
        q_t = \sin (t/10\pi),\ r_t = \sin (t/20\pi).
        \label{eq_loss_1}
    \end{equation}
    \item Step weights defined as 
    \begin{equation}
        \begin{aligned}
            (q_t, r_t) = \left\{ \begin{array}{cc} \left(\frac{\log(2)}{2}, 1 \right)  , \ & t \leq T/5,  \\ 
            \left(1, 1 \right) , \ & T/5 < t \leq 2T/5, \\
            \left(\frac{\log(2)}{2}, \frac{\log(2)}{2} \right)  , \ & 2T/5 < t \leq 3T/5, \\  
            \left(1, \frac{\log(2)}{2} \right)  , \ & 3T/5 < t \leq 4T/5,  \\
            \left(\frac{\log(2)}{2}, 1 \right)   , \ & 4T/5 < t \leq T.
            \end{array} \right.
        \end{aligned}
        \label{eq_loss_2}
    \end{equation}
\end{enumerate}

\myParagraph{Results} 
The results are summarized in \Cref{table_OCOvsOCOM_single} and \Cref{table_OCOvsOCOM_hedge}, showing that \SafeOGD and \SafeAder controllers outperform \DAC and \Scream controllers in terms of average and standard deviation of cumulative loss under various noise distributions. \SafeOGD and \SafeAder controllers have comparable performance against \DAC and \Scream under Gaussian, Uniform, and Beta distributions, and achieve significant improvements under Gamma, Exponential, and Weibull distributions.
